# Supplementary material for: TSTR: Too Short to Represent, Summarize with Details! Intro-Guided Extended Summary Generation
Source: arXiv:2206.00847 source file (2022-06-02)
Supplement: Supplementary file 1 [file appendix.tex]

\section*{appendix}
